# Supplementary material for: A General Framework for Distributed Partitioned Optimization
Source: arXiv:2203.00681 source file (2023-01-29)
Supplement: Supplementary file 1 [file appendix_draft.tex]

\section{Appendix}

\subsection{Eigenvalues of ring-clique graph }
\label{ring-clique_eigenvalues}


 \begin{center}
\begin{figure}[h!]
\centering
\includegraphics[width=0.6\linewidth]{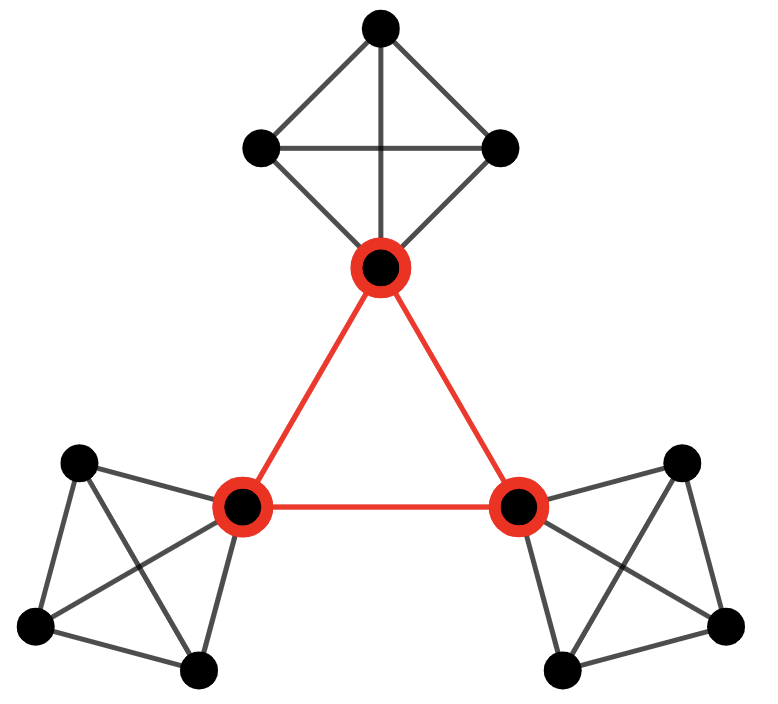}
\caption{An example of ring-clique graph with three 4-vertices graphs}

\label{fig:1}

\end{figure}
\end{center}



If the laplacian of the clique is $\mL$ and  $\textbf{0}$ is $0$-vector of size $k$, then define:

\begin{align*}
    \mL' = 
    \begin{bmatrix}
        & 2 & \textbf{0}^T \\
        & \textbf{0}& \mL \\
        \end{bmatrix}
\end{align*}

and 

\begin{align*}
    \mU = 
    \begin{bmatrix}
        &\text{-}1 & 0& \cdots & 0 \\
        & 0 & 0& \cdots & \vdots \\
        &\vdots & \vdots& \ddots&\vdots \\
        & 0& \cdots&\cdots &  0\\
        \end{bmatrix}
\end{align*}



Figure \eqref{fig:1} is an example of ring-clique graph that consists of $3$ crowns. 
Its laplacian $\bf{\Lambda}$ has the following form:

 
 \begin{eqnarray*}
    C=\left[
\begin{array}{c | c | c}
\mL' & \mU & \mU \\ \hline
\mU & \mL' & \mU \\ \hline
\mU & \mU & \mL' \\ 
\end{array}\right]
 \end{eqnarray*}

Let matrix $\mC$ in general be the following:


\begin{eqnarray*}
    \mC = 
    \begin{bmatrix*}[r]
        &2 &\text{-}1 & 0 & \cdots & \cdots & \cdots  & \text{-}1\\
        &\text{-}1 &2 & \text{-}1 & 0 & \cdots & \cdots  & 0\\
        &0 &\text{-}1 & 2 & \text{-}1 & 0 & \cdots  & 0\\
        &\vdots &0 & \text{-}1 & \ddots & \text{-}1 & \cdots  & \vdots\\
        &\vdots &\vdots & 0 & \text{-}1 & \ddots & \text{-}1  & \vdots\\
        &0 &0 & \vdots & 0 & \text{-}1 & \ddots  & \vdots\\
        &\text{-}1 & 0 & 0 & \cdots & 0 & \text{-}1  & 2\\
        \end{bmatrix*}
\end{eqnarray*}

In the case of $3$ cliques:

\begin{eqnarray*}
    \mC = 
    \begin{bmatrix*}[r]
        & 2 & \text{-}1 & \text{-}1 \\
        & \text{-}1 & 2 & \text{-}1 \\
        & \text{-}1 & \text{-}1 & 2 \\
        \end{bmatrix*}
\end{eqnarray*}



Matrix $\mB = \textbf{h}^T \cdot \textbf{h}$, where $\textbf{h} = \left[1, 0, \ldots, 0 \right]$

Then 

\begin{eqnarray*}
    \bf{\bf{\Lambda}} = \mI_n \otimes \mL + \mC \otimes \mB\\
\end{eqnarray*}

To obtain the eigenvalues of $\bf{\Lambda}$, we need to diagonalize it. 
Let $\mC = \mS^{-1} \Psi \mS, \; \Psi = \text{diag} \left(\lambda_1, \lambda_2, \ldots, \lambda_n \right)$. ($\lambda_i$ is eigenvalue of matrix $\mC$)

Then 
\begin{eqnarray*}
    \hat{\bf{\Lambda}} = \left( \mS \otimes \mI_k \right)^{-1} \bf{\Lambda} \left( \mS \otimes \mI_k \right)
\end{eqnarray*}

 and, finally, 
 
 \begin{eqnarray*}
    \hat{\bf{\Lambda}} = \mI_n \otimes \mL + \Psi \otimes \mB
 \end{eqnarray*}
 
 or (in the case of $3$ cliques)
  
  \begin{eqnarray*}
\hat{\bf{\Lambda}} =
\begin{bmatrix}
\mL & & \\
 & \mL & \\
 &  & \mL
\end{bmatrix}
+
\begin{bmatrix}
\lambda_1 \mB & & \\
 & \lambda_2 \mB & \\
 &  & \lambda_3 \mB
\end{bmatrix}
\end{eqnarray*} (where empty spaces are filled with $0$) and 
  
   \begin{eqnarray*}
\hat{\bf{\Lambda}} =
\begin{bmatrix}
\mL & & \\
 & \ddots & \\
 &  & \mL
\end{bmatrix}
+
\begin{bmatrix}
\lambda_1 \mB & & \\
 & \ddots  & \\
 &  & \lambda_n \mB
\end{bmatrix}
\end{eqnarray*}
 in general case. 
 
 To find the eigenvalues $\theta_j^i$, we write the equation
 
 
 \begin{eqnarray*}
\hat{\bf{\Lambda}} 
\begin{bmatrix}
x_1 \\
\vdots \\
x_n
\end{bmatrix}
=
\begin{bmatrix}
 \left(\mL + \lambda_1 \mB \right) x_1  \\
\vdots  \\
\left(\mL + \lambda_n \mB \right) x_n  
\end{bmatrix}
= \theta_j 
\begin{bmatrix}
 x_1 \\
 \vdots \\
 x_n
\end{bmatrix}
\end{eqnarray*}

Now, using Lemma \eqref{lemma1}, we obtain that
\begin{eqnarray*}
    \chi(\hat{\bf{\Lambda}}) = \dfrac{\max\limits_i{\lambda_{\text{max}} (\mL + \lambda_i \mB})}{\min\limits_i{\lambda^+_{\text{min}} (\mL + \lambda_i \mB})}
\end{eqnarray*}

To find the eigenvalues of matrices $\mL + \lambda_i \mB$, let fix some $\lambda_i = \lambda$ and write:

\begin{eqnarray*}
    \mL + \lambda \cdot \mB = 
    \begin{bmatrix*}[r]
        &k-1+\lambda-\theta&\text{-}1&\cd&\cd&\text{-}1 \\
        &\text{-}1&k-1-\theta&\text{-}1&\cd&\text{-}1 \\
        &\vd&\text{-}1&\ddots&\ddots&\vd \\
        &\vd&\vd&\ddots&\ddots&\text{-}1 \\
        &\text{-}1&\text{-}1&\cd&\text{-}1&k-1-\theta \\
        \end{bmatrix*}
\end{eqnarray*}

Let 

\begin{eqnarray*}
    \bf{u} = 
    \begin{bmatrix}
        & 1  &\cdots &1  \\
        \end{bmatrix}
\end{eqnarray*}

\begin{eqnarray*}
    \bf{v} = 
    \begin{bmatrix}
        & \text{-}1  & \cdots &\text{-}1  \\
        \end{bmatrix}
\end{eqnarray*}

Represent $\mL + \lambda \cdot \mB$ in the form:

$\mL + \lambda \cdot \mB = \mA + \bf{uv}^T $, hence 



\begin{eqnarray*}
    \mA = 
    \begin{bmatrix}
        &k+\lambda-\theta&0&\cd&\cd&0 \\
        &0&k-\theta&0&\cd&0 \\
        &\vd&0&\ddots&\ddots&\vd \\
        &\vd&\vd&\ddots&\ddots&0 \\
        &0&0&\cd&0&k-\theta \\
        \end{bmatrix}
\end{eqnarray*}

According to matrix determinant lemma (see Lemma $1.1$ from \cite{ding2007eigenvalues}):

\begin{eqnarray*}
    \text{det} \left( \mA + \bf{uv}^t \right) = \left( 1 + \bf{v}^T \cdot \mA^{-1} \cdot  \bf{u} \right) \cdot \text{det} \mA
\end{eqnarray*}


\begin{eqnarray*}
    \mA^{-1} = 
    \begin{bmatrix}
        &\dfrac{1}{k+\lambda-\theta}&0&\cd&\cd&0 \\
        &0&\dfrac{1}{k-\theta}&0&\cd&0 \\
        &\vd&0&\ddots&\ddots&\vd \\
        &\vd&\vd&\ddots&\ddots&0 \\
        &0&0&\cd&0&\dfrac{1}{k-\theta} \\
        \end{bmatrix}
\end{eqnarray*}



\begin{eqnarray*}
    \bf{v}^T \cdot \mA^{-1} = 
    \begin{bmatrix}
        & \dfrac{1}{k+\lambda-\theta}  & \dfrac{1}{k-\theta}  &\cdots   & \dfrac{1}{k-\theta} \\
        \end{bmatrix}
\end{eqnarray*}

%\begin{align*}
%    \m{\bf{v}^T \cdot \text{A}^{-1}\cdot  \bf{u}} = 
 %%       & $-\dfrac{1}{k+\lambda-\theta} - \dfrac{k-1}{k-\theta}$ \\
 %%\end{align*}

$\bf{v}^T \cdot \mA^{-1}\cdot  \bf{u}$  $= -\dfrac{1}{k+\lambda-\theta} - \dfrac{k-1}{k-\theta}$

$1 +\bf{v}^T \cdot \mA^{-1}\cdot  \bf{u}$  $= 1 -\dfrac{1}{k+\lambda-\theta} - \dfrac{k-1}{k-\theta}$ 




\begin{eqnarray*}
    \text{det} \;  \hat{\bf{\Lambda}} &=& \left[ 1 -\dfrac{1}{k+\lambda-\theta} - \dfrac{k-1}{k-\theta} \right] (k + \lambda - \theta) (k-\theta)^{k-1}  \nonumber \\
    &&= (k+\lambda-\theta)(k-\theta)^{k-1} - (k-\theta)^{k-1} - (k-1)(k+\lambda-\theta) (k-\theta)^{k-2} \nonumber \\
    &&= (k-\theta)^{k-2} \cdot \left[ (k + \lambda - \theta) \cdot (k-\theta) - (k-\theta) - (k-1)(k+\lambda-\theta) \right] \nonumber \\
    &&= (k-\theta)^{k-2} \left[ \theta^2 + \theta(-k-\lambda) + \lambda \right] \nonumber \\
    &&= (k-\theta)^{k-2} \left[ \theta - \theta_1 \right]\left[ \theta - \theta_2 \right]
    \end{eqnarray*}
    
    
Now we obtain the eigenvalues of ring-clique graph:

\begin{enumerate}
    \item[$1)$] $\theta_1 = \dfrac{k+\lambda + \sqrt{\lambda^2 + 2(k-2)\lambda+k^2}}{2} $
    
    \item[$2)$] $\theta_2= \dfrac{k+\lambda - \sqrt{\lambda^2 + 2(k-2)\lambda+k^2}}{2} $
    
    \item[$3)$]  $\theta_{3\ldots k } = k$
\end{enumerate}
    
    
    
    
   


\subsection{Spectrum of $\hat{\bf{\Lambda}}$ assumption}
\label{spectrum_lambda_assumption}
\begin{lemma}
\label{lemma1}

\end{lemma}

\subsection{Asymptotics of the condition number of laplacian of ring-clique graph}
\label{condition_number_asymptotics}

\begin{theorem}
\label{cond_numb_asymptotics_ring_clique}
Condition number $\chi(\bf{\bf{\Lambda}})$ of laplacian of ring-clique graph has asymptotics $\Theta (n^2 k^2)$

\end{theorem}

\textbf{Proof:}

Combining \eqref{ring-clique_eigenvalues} and \eqref{spectrum_lambda_assumption} results and, since $\lambda_i \in \left[0, 4 \right]$

\begin{eqnarray*}
    \theta_{\text{max}} = \dfrac{k + 4 + \sqrt{16 + 8(k-2) + k^2}}{2} \sim \Theta(k)
\end{eqnarray*}

To find the $\theta_{\text{min}}$ estimate, we need to show, that $\theta_2(\lambda)$ from \eqref{ring-clique_eigenvalues} is an increasing function. 

\begin{eqnarray*}
    \theta'_2(\lambda) = \dfrac{-k-\lambda+2}{2\sqrt{k^2 + \lambda^2 + 2(k-2)\lambda}} + \dfrac{1}{2}
\end{eqnarray*}

Since $k \geq 2$, then $k+\lambda - 2 \leq \sqrt{k^2 + \lambda^2 + 2(k-2)\lambda}$, then $\theta'_2(\lambda) > 0$ and $\theta^+_{\text{min}}(\lambda)$ is reached at the $\max{\cos{\dfrac{2\pi i}{n}}} \neq 1$, that is $i = 1$. 

Then 

\begin{eqnarray*}
    \theta_{\text{min}}^+ = \dfrac{1}{2} \left[ k + 2 - 2 \cos{\dfrac{2\pi}{n}} - \sqrt{4\left(1-\cos{\dfrac{2\pi}{n}}\right)^2 + 4(k-2)\left(1-\cos{\dfrac{2\pi}{n}}\right) + k^2} \right]
\end{eqnarray*}

Its Taylor expansion:

\begin{eqnarray*}
    \theta_{\text{min}}^+ \sim 4\dfrac{\pi^2}{n^2 k} + o\left(\dfrac{1}{n^3}\right)
\end{eqnarray*}

Using it, we obtain:

\begin{eqnarray*}
    \theta_{\text{min}}^+ \sim  \Theta \left(  \dfrac{1}{n^2k}  \right)
\end{eqnarray*}

And, finally, 

\begin{eqnarray*}
    \chi \left(\bf{\Lambda} \right) \sim \Theta\left(  n^2 k^2  \right)
\end{eqnarray*}

\subsection{Crown-graph eigenvalues}
\label{crown_graph_eigenvalues}

 \begin{center}
\begin{figure}[h!]
\centering
\includegraphics[width=0.6\linewidth]{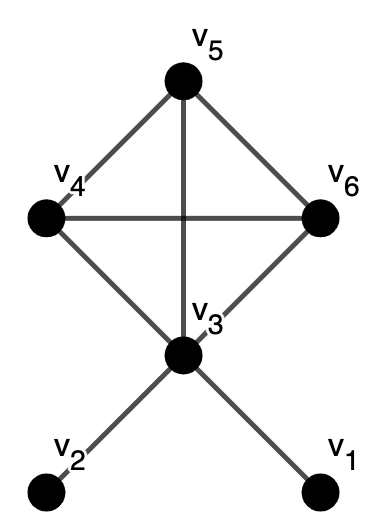}
\caption{An example of crown graph with 4 vertices ($k = 4$)}

\label{fig:2}

\end{figure}
\end{center}



In general, crown-graph laplacian has the following form:

\begin{eqnarray}
\label{cgm}
\begin{bmatrix}
    &1&0&\text{-}1&0&\cdots&0 \\
    &0&1&\text{-}1&0&\cdots&0 \\
    &\text{-}1&\text{-}1&k+1&\text{-}1&\cdots&\text{-}1 \\
    &0&0&\text{-}1&k-1&\cdots&\text{-}1 \\
    &\cdots&\cdots&\cdots&\cdots&\ddots&\cdots \\
    &0&0&\text{-}1&\text{-}1&\cdots&k\text{-}1 \\
\end{bmatrix}
\end{eqnarray}



Crown-graph complement matrix:

\begin{eqnarray}
\label{cgcm}
\begin{bmatrix}
    &k&\text{-}1&\text{-}1&\cdots&\cdots&\text{-}1&0 \\
    &\text{-}1&k&\text{-}1&\cd&\cd&\text{-}1&\vd \\
    &\text{-}1&\text{-}1&2&0&\cd&0&\vd \\
    &\vd&\vd&0&\ddots&&\vd&\vd \\
    &\vd&\vd&\vd&&\ddots&0&\vd \\
    &\text{-}1&\text{-}1&0&\cd&0&2&\vd \\
    &0&\cd&\cd&\cd&\cd&\cd&0 \\
\end{bmatrix}
\end{eqnarray}

First we will find the eigenvalues of \eqref{cgcm}.

Then 

\begin{eqnarray}
\label{det1}
\text{det}
\begin{bmatrix}
    &k-\lambda&\text{-}1&\text{-}1&\cdots&\cdots&\text{-}1 \\
    &\text{-}1&k-\lambda&\text{-}1&\cd&\cd&\text{-}1 \\
    &\text{-}1&\text{-}1&2-\lambda&0&\cd&0 \\
    &\vd&\vd&0&\ddots&&\vd \\
    &\vd&\vd&\vd&&\ddots&0 \\
    &\text{-}1&\text{-}1&0&\cd&0&2-\lambda \\
    \end{bmatrix}
    = 0
\end{eqnarray}

Using linear conversions:

\begin{eqnarray*}
    &&
    \begin{bmatrix}
    &k\text{-}\lambda&\text{-}1&\text{-}1&\cdots&\cdots&\text{-}1 \\
    &\text{-}1&k\text{-}\lambda&\text{-}1&\cd&\cd&\text{-}1 \\
    &\text{-}1&\text{-}1&2\text{-}\lambda&0&\cd&0 \\
    &\vd&\vd&0&\ddots&&\vd \\
    &\vd&\vd&\vd&&\ddots&0 \\
    &\text{-}1&\text{-}1&0&\cd&0&2\text{-}\lambda \\
    \end{bmatrix}
    \sim
    \begin{bmatrix}
    &k-\lambda+1&\text{-}1&\text{-}1&\cdots&\cdots&\text{-}1 \\
    &\lambda-k\text{-}1&k-\lambda&\text{-}1&\cd&\cd&\text{-}1 \\
    &0&\text{-}1&2-\lambda&0&\cd&0 \\
    &\vd&\vd&0&\ddots&&\vd \\
    &\vd&\vd&\vd&&\ddots&0 \\
    &0&\text{-}1&0&\cd&0&2-\lambda \\
    \end{bmatrix}\\\nonumber
    &\sim&
    \begin{bmatrix}
    &2k-2\lambda+2&\lambda-k\text{-}1&0&\cdots&\cdots&0 \\
    &\lambda-k\text{-}1&k-\lambda&\text{-}1&\cd&\cd&\text{-}1 \\
    &0&\text{-}1&2-\lambda&0&\cd&0 \\
    &\vd&\vd&0&\ddots&&\vd \\
    &\vd&\vd&\vd&&\ddots&0 \\
    &0&\text{-}1&0&\cd&0&2-\lambda \\
    \end{bmatrix}
\end{eqnarray*}

Then 

\begin{eqnarray*}
&&
\text{det}
\begin{bmatrix}
    &k\text{-}\lambda&\text{-}1&\text{-}1&\cdots&\cdots&\text{-}1 \\
    &\text{-}1&k\text{-}\lambda&\text{-}1&\cd&\cd&\text{-}1 \\
    &\text{-}1&\text{-}1&2\text{-}\lambda&0&\cd&0 \\
    &\vd&\vd&0&\ddots&&\vd \\
    &\vd&\vd&\vd&&\ddots&0 \\
    &\text{-}1&\text{-}1&0&\cd&0&2\text{-}\lambda \\
    \end{bmatrix}\\\nonumber
    &=&
    (2k-2\lambda+2)
    \begin{vmatrix}
    &k\text{-}\lambda&\text{-}1&\cd&\cd&\text{-}1 \\
    &\text{-}1&2\text{-}\lambda&0&\cd&0 \\
    &\vd&0&\ddots&&\vd \\
    &\vd&\vd&&\ddots&0 \\
    &\text{-}1&0&\cd&0&2\text{-}\lambda \\   
    \end{vmatrix}
     - (\lambda-k-1)
     \begin{vmatrix}
    &\lambda\text{-}k\text{-}1&\text{-}1&\cd&\cd&\text{-}1 \\
    &0&2\text{-}\lambda&0&\cd&0 \\
    &\vd&0&\ddots&&\vd \\
    &\vd&\vd&&\ddots&0 \\
    &0&0&\cd&0&2\text{-}\lambda \\     
     \end{vmatrix}
\end{eqnarray*}

For the second term:
\begin{eqnarray*}
    \begin{vmatrix}
    &\lambda\text{-}k\text{-}1&\text{-}1&\cd&\cd&\text{-}1 \\
    &0&2\text{-}\lambda&0&\cd&0 \\
    &\vd&0&\ddots&&\vd \\
    &\vd&\vd&&\ddots&0 \\
    &0&0&\cd&0&2\text{-}\lambda \\     
     \end{vmatrix} = (\lambda-k\text{-}1)(2-\lambda)^{k-1}
\end{eqnarray*}

For the first term we have:

\begin{eqnarray*}
    &&
   \begin{vmatrix}
    &k\text{-}\lambda&\text{-}1&\cd&\cd&\text{-}1 \\
    &\text{-}1&2\text{-}\lambda&0&\cd&0 \\
    &\vd&0&\ddots&&\vd \\
    &\vd&\vd&&\ddots&0 \\
    &\text{-}1&0&\cd&0&2\text{-}\lambda \\   
    \end{vmatrix}\\\nonumber
    &=&
    (k-\lambda)(2-\lambda)^{k\text{-}1}
    -
    (-1) \cdot 
    \begin{vmatrix}
     &\text{-}1&0&\cdots&0 \\
     &\text{-}1&2\text{-}\lambda&\cdots&0 \\
     &\vdots&\vdots&\ddots&\vdots \\
     &\text{-}1&0&\cdots&2\text{-}\lambda \\
    \end{vmatrix}
    +
    (-1) \cdot
    \begin{vmatrix}
     &\text{-}1&2-\lambda&0&\cdots&0 \\
     &\vdots&0&0&\cdots&0 \\
     &\vdots&\vdots&2\text{-}\lambda&&\vdots \\
     &\vdots&\vdots&&\ddots&0 \\
     &\text{-}1&0&\cdots&0&2\text{-}\lambda \\
    \end{vmatrix}
    -(-1) \cdot \ldots \\\nonumber
    &&=
    (k-\lambda) \cdot (2-\lambda)^{k-1} - (k-1)\cdot(2-\lambda)^{k-2} 
\end{eqnarray*}

Then, from \eqref{det1}, we have:

\begin{eqnarray*}
    (2k-2\lambda+2)\cdot\left( (k-\lambda)\cdot(2-\lambda)^{k-1}-(k-1)(2-\lambda)^{k-2} \right) - (\lambda - k - 1)^2 (2-\lambda)^{k-1} = 0
\end{eqnarray*}

\begin{eqnarray*}
    && (2k-2\lambda+2)\cdot\left( (k-\lambda)\cdot(2-\lambda)^{k-1}-(k-1)(2-\lambda)^{k-2} \right) - (\lambda - k - 1)^2 (2-\lambda)^{k-1} \\ \nonumber 
    &&= \left[ (k-\lambda+1)(2-\lambda)^{k-2} \right] \cdot \left[ 2(k-\lambda)(2-\lambda) - 2(k-1) - (k-\lambda-1)(2-\lambda) \right] \\ \nonumber
    &&= \left[ (k-\lambda+1)(2-\lambda)^{k-2} \right] \cdot \left[ \lambda(\lambda-k-1) \right] = 0
\end{eqnarray*}

Then 
\begin{enumerate}
    \item[$1)$] $\lambda_1 = 0$ 
    
    \item[$2)$] $\lambda_2 = 2$ of multiplicity $k-2$ 
    
    \item[$3)$] $\lambda_3 = k+1$ of multiplicity $2$

\end{enumerate}
are the eigenvalues of \eqref{cgcm} and, using  formula $2.2.22$ from \cite{pozrikidis2014introduction}, we obtain the eigenvalues of \eqref{cgm}:

\begin{enumerate}
    \item[$1)$] $\lambda_1 = 0$ of multiplicity $1$
    
    \item[$2)$] $\lambda_2 = 1$ of multiplicity $2$ 
    
    \item[$3)$] $\lambda_3 = k$ of multiplicity $k\--  2$
    
    \item[$4)$] $\lambda_4 = k+2$ of multiplicity $1$
\end{enumerate}

\subsection{Semi-crown graph eigenvalues}
\label{semi_crown_graph_eigenvalues}

\begin{center}
\begin{figure}[h!]
\centering
\includegraphics[width=0.6\linewidth]{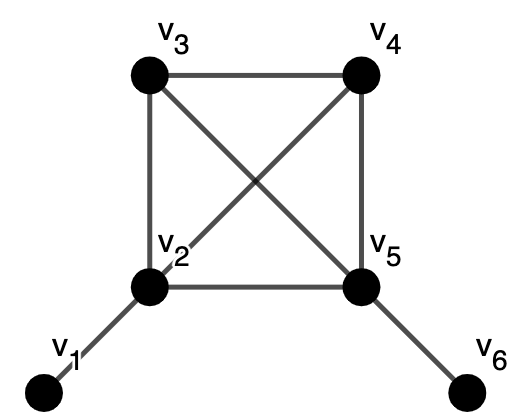}
\caption{An example of semi-crown graph with 4 vertices ($k = 4$)}

\label{fig:4}

\end{figure}
\end{center}


In general, semi-crown graph laplacian has the following form:

\begin{eqnarray}
\label{scgm}
\begin{bmatrix}
    &1&\text{-}1&0&\cd&\cd&\cd&0 \\
    &\text{-}1&l&\text{-}1&\cd&\cd&\text{-}1&\vd \\
    &0&\text{-}1&k\text{-}1&\text{-}1&\cd&\vd&\vd \\
    &\vd&\vd&\text{-}1&\ddots&\text{-}1&\vd&\vd \\
    &\vd&\vd&\vd&\text{-}1&k\text{-}1&\text{-}1&0 \\
    &\vd&\text{-}1&\cd&\cd&\text{-}1&k&\text{-}1 \\
    &0&\cd&\cd&\cd&0&\text{-}1&1 \\
\end{bmatrix}
\end{eqnarray}



Semi-crown graph complement matrix:


\begin{eqnarray}
\label{scgcm}
\begin{bmatrix}
    &k&\text{-}1&\text{-}1&\cd&\cd&\text{-}1&0 \\
    &\text{-}1&k&0&\text{-}1&\cd&\cd&\text{-}1 \\
    &\text{-}1&0&\text{-}1&0&\cd&\cd&0 \\
    &\vd&\text{-}1&0&2&\ddots&&\vd \\
    &\vd&\vd&\vd&\ddots&\ddots&0&\vd \\
    &\text{-}1&\vd&\vd&&0&2&0 \\
    &0&\text{-}1&0&\cd&\cd&0&1 \\
\end{bmatrix}
\end{eqnarray}

First we will find the eigenvalues of \eqref{scgcm}.

Then 
\begin{eqnarray}
\label{det2}
\begin{vmatrix}
    &k\text{\text{-}}\lambda&\text{-}1&\text{-}1&\cd&\cd&\text{-}1&0 \\
    &\text{-}1&k\text{-}\lambda&0&\text{-}1&\cd&\cd&\text{-}1 \\
    &\text{-}1&0&1\text{-}\lambda&0&\cd&\cd&0 \\
    &\vd&\text{-}1&0&2\text{-}\lambda&\ddots&&\vd \\
    &\vd&\vd&\vd&\ddots&\ddots&0&\vd \\
    &\text{-}1&\vd&\vd&&0&2\text{-}\lambda&0 \\
    &0&\text{-}1&0&\cd&\cd&0&1\text{-}\lambda \\
\end{vmatrix} = 0
\end{eqnarray}


\begin{eqnarray*}
&&
\begin{vmatrix}
    &k\text{-}\lambda&\text{-}1&\text{-}1&\cd&\cd&\text{-}1&0 \\
    &\text{-}1&k\text{-}\lambda&0&\text{-}1&\cd&\cd&\text{-}1 \\
    &\text{-}1&0&1\text{-}\lambda&0&\cd&\cd&0 \\
    &\vd&\text{-}1&0&2\text{-}\lambda&\ddots&&\vd \\
    &\vd&\vd&\vd&\ddots&\ddots&0&\vd \\
    &\text{-}1&\vd&\vd&&0&2\text{-}\lambda&0 \\
    &0&\text{-}1&0&\cd&\cd&0&1\text{-}\lambda \\
\end{vmatrix} \\ \nonumber
&&=
\begin{vmatrix}
    &k-\lambda+1&\lambda-k-1&\text{-}1&0&\cd&0&1 \\
    &\text{-}1&k-\lambda&0&\text{-}1&\cd&\cd&\text{-}1 \\
    &\text{-}1&0&1-\lambda&0&\cd&\cd&0 \\
    &\vd&\text{-}1&0&2-\lambda&\ddots&&\vd \\
    &\vd&\vd&\vd&\ddots&\ddots&0&\vd \\
    &\text{-}1&\vd&\vd&&0&2-\lambda&0 \\
    &0&\text{-}1&0&\cd&\cd&0&1-\lambda \\
\end{vmatrix} \\ \nonumber
&&= 
\begin{vmatrix}
    &2k-2\lambda+2&\lambda-k-1&\text{-}1&0&\cd&0&1 \\
    &\lambda-k-1&k-\lambda&0&\text{-}1&\cd&\cd&\text{-}1 \\
    &\text{-}1&0&1-\lambda&0&\cd&\cd&0 \\
    &0&\text{-}1&0&2-\lambda&\ddots&&\vd \\
    &\vd&\vd&\vd&\ddots&\ddots&0&\vd \\
    &0&\vd&\vd&&0&2-\lambda&0 \\
    &1&\text{-}1&0&\cd&\cd&0&1-\lambda \\
\end{vmatrix} \\ 
\end{eqnarray*}

\begin{eqnarray*}
    &&=
\begin{vmatrix}
    &2k-2\lambda+2-\dfrac{2}{1-\lambda}&\lambda-k-1+\dfrac{1}{1-\lambda}&0&\cd&\cd&0&0 \\
    &\lambda-k-1&k-\lambda&0&\text{-}1&\cd&\cd&\text{-}1 \\
    &\text{-}1&0&1-\lambda&0&\cd&\cd&0 \\
    &0&\text{-}1&0&2-\lambda&\ddots&&\vd \\
    &\vd&\vd&\vd&\ddots&\ddots&0&\vd \\
    &0&\vd&\vd&&0&2-\lambda&0 \\
    &1&\text{-}1&0&\cd&\cd&0&1-\lambda \\
\end{vmatrix} \\ \nonumber
&&=
\begin{vmatrix}
    &2k-2\lambda+2-\dfrac{2}{1-\lambda}&\lambda-k-1+\dfrac{1}{1-\lambda}&0&\cd&\cd&0&0 \\
    &\lambda-k-1+\dfrac{1}{1-\lambda}&k-\lambda&0&\text{-}1&\cd&\cd&-1 \\
    &0&0&1-\lambda&0&\cd&\cd&0 \\
    &0&\text{-}1&0&2-\lambda&\ddots&&\vd \\
    &\vd&\vd&\vd&\ddots&\ddots&0&\vd \\
    &0&\vd&\vd&&0&2-\lambda&0 \\
    &0&\text{-}1&0&\cd&\cd&0&1-\lambda \\
\end{vmatrix} \\ \nonumber
&&=
2k-2\lambda+2 - \dfrac{2}{1-\lambda}
\begin{vmatrix}
    &k\text{-}\lambda&0&\text{\text{-}}1&\cd&\cd&\text{\text{-}}1 \\
    &0&1\text{-}\lambda&0&\cd&\cd&0 \\
    &\text{\text{-}}1&0&2\text{-}\lambda&\ddots&&\vd \\
    &\vd&\vd&\ddots&\ddots&0&\vd \\
    &\vd&\vd&&0&2\text{-}\lambda&0 \\
    &\text{\text{-}}1&0&\cd&\cd&0&1\text{-}\lambda \\
\end{vmatrix} \\ \nonumber
&&- \left(\lambda-k-1+\dfrac{1}{1-\lambda}\right)
\begin{vmatrix}
    &\lambda-k-1+\dfrac{1}{1-\lambda}&0&\text{-}1&\cd&\cd&\text{-}1 \\
    &0&1-\lambda&0&\cd&\cd&0 \\
    &0&0&2-\lambda&\ddots&&\vd \\
    &\vd&\vd&\ddots&\ddots&0&\vd \\
    &0&\vd&&0&2-\lambda&0 \\
    &0&0&\cd&\cd&0&1-\lambda \\
\end{vmatrix}
\end{eqnarray*}

For the first term, we have:


\begin{eqnarray*}
&&
\begin{vmatrix}
    &k\text{-}\lambda&0&\text{-}1&\cd&\cd&\text{-}1 \\
    &0&1\text{-}\lambda&0&\cd&\cd&0 \\
    &\text{-}1&0&2\text{-}\lambda&\ddots&&\vd \\
    &\vd&\vd&\ddots&\ddots&0&\vd \\
    &\vd&\vd&&0&2\text{-}\lambda&0 \\
    &\text{-}1&0&\cd&\cd&0&1\text{-}\lambda \\
\end{vmatrix} \\ \nonumber
&&=
(k-\lambda)(1-\lambda)^2(2-\lambda)^{k-2} + (-1) \cdot 
\begin{vmatrix}
    &0&1\text{-}\lambda&0&\cd&\cd&0 \\
    &\text{-}1&0&0&\cd&\cd&0 \\
    &\vd&\vd&2\text{-}\lambda&&&\vd \\
    &\vd&\vd&&\ddots&&\vd \\
    &\vd&\vd&&&2\text{-}\lambda&0 \\
    &\text{-}1&0&\cd&\cd&0&1\text{-}\lambda \\
\end{vmatrix} - (-1) \cdots \\ \nonumber
&&= 
(k-\lambda)(2-\lambda)^2 (2-\lambda)^{k-2} - (k-2)(1-\lambda)^2
\end{eqnarray*}

For the second term:

\begin{eqnarray*}
\begin{vmatrix}
    &\lambda-k-1+\dfrac{1}{1-\lambda}&0&\text{-}1&\cd&\cd&\text{-}1 \\
    &0&1-\lambda&0&\cd&\cd&0 \\
    &0&0&2-\lambda&\ddots&&\vd \\
    &\vd&\vd&\ddots&\ddots&0&\vd \\
    &0&\vd&&0&2-\lambda&0 \\
    &0&0&\cd&\cd&0&1-\lambda \\
\end{vmatrix} = \left(\lambda-k -1 + \dfrac{1}{1-\lambda}\right) (1-\lambda)^2 (2-\lambda)^{k-2}
\end{eqnarray*}

Now, combining these results in \eqref{det2}, we have:


\begin{eqnarray*}
    2\left(k-\lambda+1 - \dfrac{1}{1-\lambda}\right) \cdot \left((k-\lambda)(2-\lambda)^2 (2-\lambda)^{k-2} - (k-2)(1-\lambda)^2 \right) - \left(\lambda-k -1 + \dfrac{1}{1-\lambda}\right)^2 (1-\lambda)^2 (2-\lambda)^{k-2} = 0
\end{eqnarray*}

The solution of this equation is the following:

\begin{enumerate}
    \item[$1)$] $\lambda_1 = 0$ of multiplicity $1$
    
    \item[$2)$] $\lambda_2 = 2$ of multiplicity $k\--3$ 
    
    \item[$3)$] $\lambda_{3, 4} = \dfrac{k+2\pm \sqrt{k^2+4}}{2}$ of multiplicity $1$
    
    \item[$4)$] $\lambda_{5,6} = \dfrac{k+2 \pm \sqrt{k^2-4}}{2}$ of multiplicity $1$
\end{enumerate}

and, using  formula $2.2.22$ from \cite{pozrikidis2014introduction}, we obtain the eigenvalues of \eqref{scgm}:

\begin{enumerate}
    \item[$1)$] $\lambda_1 = 0$ of multiplicity $1$
    
    \item[$2)$] $\lambda_2 = k$ of multiplicity $k\--3$ 
    
    \item[$3)$] $\lambda_{3, 4} = \dfrac{k+2\pm \sqrt{k^2+4}}{2}$ of multiplicity $1$
    
    \item[$4)$] $\lambda_{5,6} = \dfrac{k+2 \pm \sqrt{k^2-4}}{2}$ of multiplicity $1$
\end{enumerate}

\iffalse
\subsection{for rogoza}

%full graph
\begin{eqnarray*}
\mathcal{W} = 
\begin{bmatrix}
    &2&-1&1 \\ 
    &-1&1&0 \\ 
    &-1&0&1 \\ 
\end{bmatrix}
\end{eqnarray*}

%blue subgraph
\begin{eqnarray*}
\widetilde{\mathcal{W}}^1 = 
\begin{bmatrix}
    &1&-1 \\
    &-1&1 \\
\end{bmatrix}
\end{eqnarray*}

\begin{eqnarray*}
\mathcal{W}^1 = 
\begin{bmatrix}
    &1&-1&0 \\
    &-1&1&0 \\
    &0&0&0 \\
\end{bmatrix}
\end{eqnarray*}

%green subgraph
\begin{eqnarray*}
\widetilde{\mathcal{W}}^2 = 
\begin{bmatrix}
    &1&-1 \\
    &-1&1 \\
\end{bmatrix}
\end{eqnarray*}

\begin{eqnarray*}
\mathcal{W}^2 = 
\begin{bmatrix}
    &1&0&-1 \\
    &0&0&0 \\
    &-1&0&1 \\
\end{bmatrix}
\end{eqnarray*}

\begin{eqnarray*}
\begin{bmatrix}
    &1&0&-1&0&0&0 \\
    &0&1&0&0&0&-1 \\
    &-1&0&1&0&0&0 \\
    &0&0&0&0&0&0 \\
    &0&0&0&0&0&0 \\
    &0&-1&0&0&0&1 \\
\end{bmatrix}
\end{eqnarray*}
 \fi

\subsection{Crown-graph condition number asymptotics}

To estimate the condition number asymptotics of crown-graph, we need to find the eigenvalues of its laplacian. We do this by special technique described in \cite{pozrikidis2014introduction}.

\begin{lemma}\label{lem:crown-graph_cond_number}
The condition number of crown-graph has asymptotics $\Theta(k)$
\begin{pf}
    Firstly, to find the eigenvalues of crown-graph, we will find the eigenvalues of its complement, which has the following form:
    
    \begin{align*}
    \toxandr{\mL' \left( Cr_4 \right)} =
        \begin{bmatrix}
    &k&\text{-}1&\text{-}1&\cdots&\cdots&\text{-}1&0 \\
    &\text{-}1&k&\text{-}1&\cd&\cd&\text{-}1&\vd \\
    &\text{-}1&\text{-}1&2&0&\cd&0&\vd \\
    &\vd&\vd&0&\ddots&&\vd&\vd \\
    &\vd&\vd&\vd&&\ddots&0&\vd \\
    &\text{-}1&\text{-}1&0&\cd&0&2&\vd \\
    &0&\cd&\cd&\cd&\cd&\cd&0 \\
        \end{bmatrix}
    \end{align*}
    Hence, we have
    
    \begin{align*}
        \text{det} \left( \mL' \left( Cr_4 \right) - \lambda \mI_{k+2} \right) = 0
    \end{align*}
    
    which, through linear conversions, leads us to the equation 
    
    \begin{align*}
        \left[ (k-\lambda+1)(2-\lambda)^{k-2} \right] \cdot \left[ \lambda(\lambda-k-1) \right] = 0
    \end{align*}
    
    Now we have the eigenvalues of crown-graph complement: 
    \begin{enumerate}
    \item[$1)$] $\lambda_1 = 0$ 
    
    \item[$2)$] $\lambda_2 = 2$ of multiplicity $k-2$ 
    
    \item[$3)$] $\lambda_3 = k+1$ of multiplicity $2$

    \end{enumerate} 
    
    And, using formula $2.2.22$ from \cite{pozrikidis2014introduction}, we obtain the eigenvalues of crown-graph:

\begin{enumerate}
    \item[$1)$] $\lambda_1 = 0$ of multiplicity $1$
    
    \item[$2)$] $\lambda_2 = 1$ of multiplicity $2$ 
    
    \item[$3)$] $\lambda_3 = k$ of multiplicity $k\--  2$
    
    \item[$4)$] $\lambda_4 = k+2$ of multiplicity $1$
\end{enumerate}
Thus, we get the asymptotics of condition number $\Theta(k)$
\end{pf}
\end{lemma}
